# Supplementary material for: "I understand why I got this grade": Automatic Short Answer Grading with Feedback
Source: arXiv:2407.12818 source file (2025-06-23)
Supplement: Supplementary file 1 [file Supplimentary_material.tex]

\documentclass{article}

% if you need to pass options to natbib, use, e.g.:
%     \PassOptionsToPackage{numbers, compress}{natbib}
% before loading neurips_data_2023

% ready for submission
\usepackage{neurips_data_2024}

% to compile a preprint version, add the [preprint] option, e.g.:
%     \usepackage[preprint]{neurips_data_2023}
% This will indicate that the work is currently under review.

% to compile a camera-ready version, add the [final] option, e.g.:
%     \usepackage[final]{neurips_data_2023}

% to avoid loading the natbib package, add option nonatbib:
%    \usepackage[nonatbib]{neurips_data_2023}

% Submissions to the datasets and benchmarks are typically non anonymous,
% but anonymous submissions are allowed. If you feel that you must submit 
% anonymously, you can compile an anonymous version by adding the [anonymous] 
% option, e.g.:
%     \usepackage[anonymous]{neurips_data_2023}
% This will hide all author names.

\usepackage[utf8]{inputenc} % allow utf-8 input
\usepackage[T1]{fontenc}    % use 8-bit T1 fonts
\usepackage{hyperref}       % hyperlinks
\usepackage{url}            % simple URL typesetting
\usepackage{booktabs}       % professional-quality tables
\usepackage{amsfonts}       % blackboard math symbols
\usepackage{nicefrac}       % compact symbols for 1/2, etc.
\usepackage{microtype}      % microtypography
\usepackage{xcolor}         % colors

% additional libraries
\usepackage{graphicx}
\usepackage{subcaption}
\usepackage{natbib}
\definecolor{ao(english)}{rgb}{0.0, 0.5, 0.0}
\usepackage{booktabs}
\usepackage{wrapfig}

\usepackage{todonotes}

\title{Supplementary Material}

% The \author macro works with any number of authors. There are two commands
% used to separate the names and addresses of multiple authors: \And and \AND.
%
% Using \And between authors leaves it to LaTeX to determine where to break the
% lines. Using \AND forces a line break at that point. So, if LaTeX puts 3 of 4
% authors names on the first line, and the last on the second line, try using
% \AND instead of \And before the third author name.

% \author{%
%   Dishank Aggarwal
%   % Department of Computer Science\\
%   % Indian Institute of Technology, Bombay\\
%   % \texttt{dishankaggarwal@cse.iitb.ac.in} \\
%   \And
%   Pushpak Bhattacharyya
%   % Department of Computer Science \\
%   % Indian Institute of Technology, Bombay\\
%   % \texttt{pb@cse.iitb.ac.in} \\
%   \And
%   Bhaskaran Raman\\
%   \AND
%   Department of Computer Science \\
%   Indian Institute of Technology, Bombay\\
%   \texttt{\{dishankaggarwal, pb, br\}@cse.iitb.ac.in} \\
%   % \And
%   % Coauthor \\
%   % Affiliation \\
%   % Address \\
%   % \texttt{email} \\
%   % \And
%   % Coauthor \\
%   % Affiliation \\
%   % Address \\
%   % \texttt{email} \\
% }

\begin{document}

\maketitle

\section{EngSAF Dataset- Courses and Subjects}
\label{courseDistribution}
EngSAFE dataset contains questions from the following courses. Our code and dataset are available at \url{https://github.com/dishankaggarwal/EngSAF}
\begin{enumerate}
\itemsep-0.5em 
\item Sustainability Assessment of Urban Systems
\item Introduction to Philosophy
\item Business Valuation, Mergers and Acquisitions
\item Environmental Management
\item Fundamentals of Environmental Chemistry
\item Environmental Chemistry
\item Municipal waste and biomedical waste management
\item Solid Waste Management - Basic Principles and Technical Aspects
\item Mechanical Behavior of Materials
\item Water Resource Engineering
\item Advanced Hydrological Analysis and Design
\item Solid and Hazardous Waste Laboratory
\item Embedded Systems
\item Water Quality Management
\item Abstractions and Paradigms for Programming
\item Manufacturing Processes
\item Operating Systems
\item Water Resources and Environmental Hydraulics
\item Fiber Reinforced Composites
\item Electrochemical Materials Science
\item Environmental Microbiology and Ecology
\item Probabilistic and Statistical Methods in Civil Engineering
\item Image Processing
\item Computer-integrated Manufacturing
\item Mass Transfer Processes in Environmental Systems

\end{enumerate}

\section{Zero-Shot Experiment Prompt}
\label{chat-gpt prompt}

The following prompt is used for the zero-shot experiment using \textbf{gpt-3.5-turbo-16k} model. 

\begin{quote}
\emph{You are an automatic short-answer feedback generator.  
} 
\end{quote}
\begin{quote}
    \emph{ Given a question, a student answer, and a reference answer. Evaluate student answers against a reference answer for correctness, providing labels (correct/partially correct/incorrect) and constructive feedback in about 3-4 lines.}
\end{quote}

\begin{quote}
    \emph{Ensure feedback guides the learner without invoking negative emotions and does not reference the provided reference answer.}
\end{quote}
\begin{quote}
    \emph{Format output with the label on the first line followed by feedback starting from the next line.}
\end{quote}

\section{More Examples}
\label{more-examples}
Table \ref{tab:Eng-SAF_example_appendix} presents two additional questions from the EngSAF dataset. Each question is accompanied by a reference answer and multiple student answers, each labeled with their respective output label and feedback summary.

\section{Oualitative Analysis}

Table \ref{tab:Qualitative-analysis} shows an example of the fine-tuned ASAG model's output on a sample from the EngSAF test set used for qualitative analysis.
The gold label classifies the student's answer as incorrect, emphasizing that the student did not address how corners benefit specific image analysis applications. The model classifies the answer as partially correct, acknowledging that the student captured the essence of what corners represent but failed to elaborate on their practical applications. The model's feedback correctly identifies the main issue with the student’s answer: it lacks specific examples of how corners are useful in image analysis applications. The reference answer provides specific applications such as image segmentation, edge detection, and object classification. The feedback suggests that the student should include these specific applications to improve his answer. This guidance is important for a complete understanding and improvement. The feedback is educational, aiming to help the student understand better by encouraging the practical uses of the concept. This helps correct the current answer and aids the student’s overall learning by showing the importance of practical applications in theoretical concepts. The distinction between an answer being incorrect or partially correct is quite subtle. Therefore, while the model predicted the student's response as partially correct, the feedback explained the assigned grade accurately.

\begin{table*}[h!]

\centering
\begin{tabular}{p{0.2\linewidth}  p{0.7\linewidth} }
\toprule
% &\multicolumn{1}{c}{\textbf{Text}} & \multicolumn{1}{c}{\textbf{Label}} \\
% \midrule
\textbf{Question 1}&Which image analysis applications benefit from interest points like corners?\\
\textbf{Reference Answer} &Harris Corner detection from the corner, we can Improve image segmentation; if we have corners, we can detect edges more efficiently. By using corner details, we can improve object classification. It is used in many Computer vision applications.
\\
% \hline
% \textbf{Max Marks} & 2\\
\textbf{Student Answer}&A corner implies that there is a change in all the directions and this change is particularly significant where helps in analysis.\\
\textbf{Gold Output Label}&\textcolor{red}{\textbf{0 (Incorrect response)}}\\
\textbf{Gold Feedback}&Your answer provides a basic definition of a corner but does not address the image analysis applications that benefit from corner detection techniques. Try to relate the characteristics of corners to specific image analysis tasks or applications where they are commonly used.
\\
\midrule

\textbf{Pred. Label}&\textcolor{blue}{\textbf{1 (Partially correct response)}}\\
\textbf{Pred. Feedback}&Your answer captures the essence of corners as points of significant change in an image. However, it does not directly address how corners benefit image analysis applications. Try to focus on the specific advantages of corners in the context of image analysis, such as improving segmentation, edge detection, and object classification.
\\

\bottomrule 
\end{tabular}

\caption{Example \#1: Output from the fine-tuned ASAG Model on a sample from the EngSAF test set.}
\label{tab:Qualitative-analysis}
\end{table*}

Table \ref{tab:Qualitative-analysis-2} shows an example of the fine-tuned ASAG model's output on a sample from the EngSAF test set used for qualitative analysis. The model's feedback accurately recognizes the comprehensiveness of the student’s answer, which aligns well with the reference answer. The student correctly notes that multilayer perceptron (MLP) networks with multiple hidden layers are beneficial for learning non-linear features and handling complex feature discrimination. The feedback is positive, acknowledging the correctness of the student’s response and providing encouragement. This accurate assessment demonstrates the model's capability to deliver meaningful and constructive feedback, crucial for the student’s learning process. By validating the student’s understanding and encouraging further exploration, the feedback contributes to a supportive educational environment.

\begin{table*}[h!]

\centering
\begin{tabular}{p{0.2\linewidth}  p{0.7\linewidth} }
\toprule
% &\multicolumn{1}{c}{\textbf{Text}} & \multicolumn{1}{c}{\textbf{Label}} \\
% \midrule
\textbf{Question 1}&Under which circumstances is a multilayer perceptron neural network with multiple hidden layers (>1 layer) desirable?\\
\textbf{Reference Answer} &when more deep learning or critical learning of features are required, then more hidden layers are required to extract out and learn features properly and efficiently so as to perform further tasks well. example- multiclass classification, XOR function.
\\
% \hline
% \textbf{Max Marks} & 2\\
\textbf{Student Answer}&it is desirable when we want to learn non-linear features. as the number of hidden layers increases, we can learn more complex, non-linear features. thus, we use it for a problem involving discrimination of complex features.
\\

\textbf{Gold Output Label}&\textcolor{ao(english)}{\textbf{2 (Correct response)}}\\
\textbf{Gold Feedback}&Your answer grasps the key concept of using multilayer perceptron neural networks with multiple hidden layers for learning complex, non-linear features. This is indeed a correct and insightful response. Keep exploring different types of neural network architectures and their applications to various problems.
\\
\midrule

\textbf{Pred. Label}&\textcolor{ao(english)}{\textbf{2 (Correct response)}}\\
\textbf{Pred. Feedback}& Your answer captures the essence of when multilayer perceptron neural networks with multiple hidden layers are desirable. It correctly highlights the purpose of increasing the number of hidden layers for learning complex, non-linear features. Well done!\\

\bottomrule 
\end{tabular}

\caption{Example \#2: Output from the fine-tuned ASAG Model on a sample from the EngSAF test set.}
\label{tab:Qualitative-analysis-2}
\end{table*}

\section{Deployment details}
For the real-world deployment, our fine-tuned ASAG model was integrated into an end-semester exam on \textbf{ET 623 (Learning Analytics Course)} at \textbf{IIT Bombay} for the 2024 academic year. The setup included the students enrolled in the course who consented to participate in the experiment. The end-sem exam includes \textbf{2} short-answer questions, each accompanied by the instructor's correct/reference answer. Table \ref{tab:deploy} contains the details of the question and reference answer. 
 Each predicted feedback is analyzed by \textbf{three Subject Matter Expert (SME)} in terms of Feedback Correctness/ Accuracy and Emotional Impact as discussed in the Quality Estimate section of the main paper. Each aspect is scored on a scale (1-5), with a high score indicating a better response. Each annotator is a current PhD student and expert in the education technology domain, ensuring the reliability of evaluations during real-world deployment of the ASAG model in the learning analytics course.

Upon evaluation, the evaluation scores greater than \textbf{4.5} (Out of 5) for both the\textbf{ Feedback Quality/Correctness} and the \textbf{Emotional Impact} aspect demonstrate the reliability and effectiveness of the ASAG model in real-world scenarios. Additionally, the model’s predicted output label achieved an accuracy of \textbf{92.5\%}, further showcasing its performance and reliability. Further, they achieved a Fleiss' Kappa score of \textbf{0.83} (Almost perfect agreement) for the \textbf{feedback quality/correctness} aspect, providing valuable insights into the agreement among three annotators in evaluating performance.

\begin{table*}[h!]

\centering
\begin{tabular}{p{0.2\linewidth}  p{0.7\linewidth} }
\toprule
% &\multicolumn{1}{c}{\textbf{Text}} & \multicolumn{1}{c}{\textbf{Label}} \\
% \midrule
\textbf{Question 1}&Explain the role of different stakeholders in learning analytics.\\
\textbf{Reference Answer}& Key stakeholders are 1) Educators, 2) Students, 3) Policymakers or Administration Educators who benefit from learning analytics by gaining real-time insights into learner performance, including identifying students who may be underperforming. This information enables educators to improve their teaching activities and methodology to meet the specific needs of individual learners, thereby improving overall teaching effectiveness. For students, learning analytics provides valuable feedback on their performance relative to their peers and progress toward personal learning goals. This feedback serves as a source of motivation and encouragement. It helps them make better decisions for their future career. Policymakers and administrators face complex challenges in the education landscape, including budget constraints and global competition. Learning analytics offers valuable data-driven insights that inform decision-making processes regarding resource allocation, curriculum development, and strategic planning. It helps significantly in improving the quality of education.\\
\midrule
\textbf{Question 2}&We have the process models below for two groups of students divided based on their final grades in a course. These are based on log data in a MOOC. Group A consists of students in the top 30 percentile; the rest are in group B. Thicker arrows mean more frequently followed paths while thinner transitions are less frequent. Based on these models, what conclusions can be drawn regarding their learning patterns and what methodology should be encouraged in the classroom? Refer to figure \ref{fig:ET623}\\

\textbf{Reference Answer}& Group A seems first to cover learning content more thoroughly - reading, watching videos, and referring/participating in discussions done in conjunction - and then proceeding to practice questions. They also refer back to course material when doing questions and then do assignments. Meanwhile, group B students focus more on practice questions and go to reading/videos in between. There is considerably less interaction with the discussions page as well. This might indicate only referring to content relevant to those questions. Thorough course content consumption should be
encouraged.\\

\bottomrule 
\end{tabular}

\caption{Two questions used to evaluate the EngSAF fine-tuned ASAG model in real-world deployment during an end-semester exam for the ET 623 (Learning Analytics Course) course at IIT Bombay. }
\label{tab:deploy}
\end{table*}

\begin{figure*}[] % Use figure* for spanning across two columns
  \centering % Center the figure
  \includegraphics[width=1\textwidth]{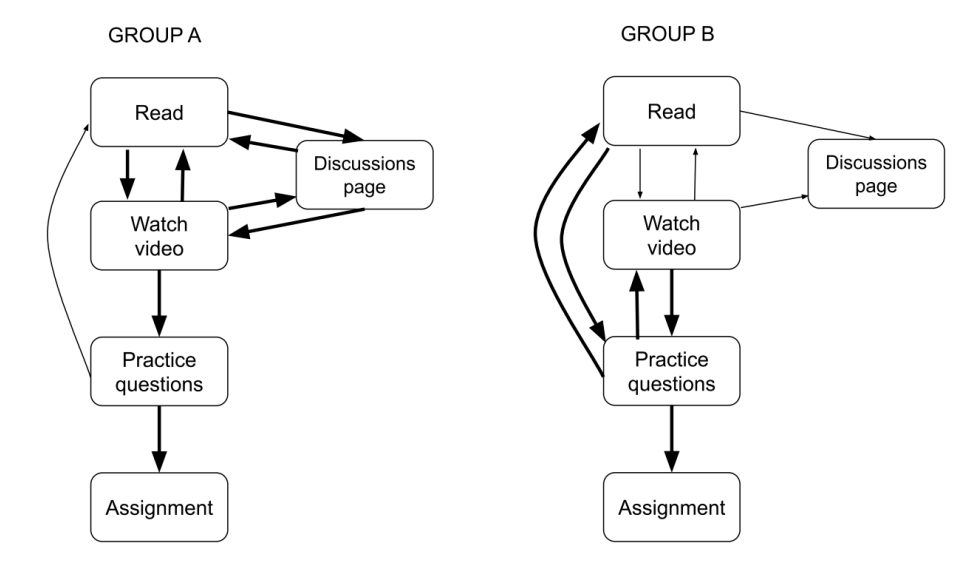} % Include your image with desired width
  \caption{Figure for Question 2 from real-world deployment} % Add your caption here
  \label{fig:ET623} % Add a label for referencing
\end{figure*}

\begin{table*}[h!]

\centering
\begin{tabular}{p{0.2\linewidth}  p{0.7\linewidth} }
\toprule
% &\multicolumn{1}{c}{\textbf{Text}} & \multicolumn{1}{c}{\textbf{Label}} \\
% \midrule
\textbf{Question 1}&What do you mean by empirical equations?\\
\midrule
\textbf{Reference Answer} &Equations derived from experiments/observed data. They don't have a mathematical proof behind them.\\
% \hline
% \textbf{Max Marks} & 2\\
\midrule
\textbf{Student Answer 1a }&The equations which are obtained through extensive experimentation involving constant numerical terms are called empirical equations.\\
\textbf{Label}&\textcolor{ao(english)}{\textbf{2 (Correct response)}}\\
\textbf{Feedback}& Well done! Your answer demonstrates a clear understanding of the concept of empirical equations. You have correctly highlighted the key characteristics of empirical equations, including their derivation from experiments and the presence of constant numerical terms.\\
\midrule
\textbf{Student Answer 1b} &these equations which are formed by empirical (experimental) data.\\
\textbf{Label}&\textcolor{blue}{\textbf{1 (Partially Correct response)}}\\
\textbf{Feedback}&Your answer is partially correct. While you mentioned the empirical nature of these equations, you missed the key point that they lack a mathematical proof. Try to include this aspect in your definition.\\
\midrule
\textbf{Student Answer 1c} &the equation which is derived for specific area of land .\\
\textbf{Label}&\textcolor{red}{\textbf{0 (Incorrect response)}}\\
\textbf{Feedback}&Empirical equations are derived from experiments or observed data across a wide range of conditions, not from a specific area of land. Consider broadening your definition to include the general concept of deriving equations from experimental data.
\\

\midrule
\midrule

\textbf{Question 2}&What issues arise when the number of hidden layers is very large?\\
\midrule
\textbf{Reference Answer} &When the number of hidden layers is very large, then the model contains a high variance, and overfitting occurs, so it cannot generalize new unseen test data but performs well on training data. Backpropagation also becomes slow.\\
% \hline
% \textbf{Max Marks} & 2\\
\midrule
\textbf{Student Answer 2a }&Issues that arise are:  Training becomes slow. If the training data is small, then the model doesn't generalize well. Also, overfitting occurs,\\
\textbf{Label}&\textcolor{ao(english)}{\textbf{2 (Correct response)}}\\
\textbf{Feedback}& Well done! Your answer demonstrates a clear understanding of the concept of empirical equations. You have correctly highlighted the key characteristics of empirical equations, including their derivation from experiments and the presence of constant numerical terms.\\
\midrule
\textbf{Student Answer 2b} &When number of hidden layers are very large it can cause overfitting and also increases the training time.\\
\textbf{Label}&\textcolor{blue}{\textbf{1 (Partially Correct response)}}\\
\textbf{Feedback}&Your answer is partially correct. While you mentioned the empirical nature of these equations, you missed the key point that they lack a mathematical proof. Try to include this aspect in your definition.\\
\midrule
\textbf{Student Answer 2c} &Error Backproparation arises when number of hidden layers is very large it means during training, error propogated back.\\
\textbf{Label}&\textcolor{red}{\textbf{0 (Incorrect response)}}\\
\textbf{Feedback}&   Your answer captures only one aspect of the challenges faced when the hidden layers are large. It doesn't mention issues like high variance, overfitting, and the impact on backpropagation speed. Try to cover all aspects of the concerns associated with a large number of hidden layers.\\
\bottomrule 
\end{tabular}

\caption{Two examples showcasing a question, reference answer, and three student answers (Student\#1, Student\#2, and Student\#3) alongside their corresponding labels and synthetically generated Feedback/Explanation for the assigned label from the Eng-SAF Dataset }
\label{tab:Eng-SAF_example_appendix}
\end{table*}

\section{Annotator Details}
We've brought in three human evaluators to ensure the EngSAF dataset output labels and artificial feedback quality and reliability. Each evaluator is working towards a master's degree, is in their final year/ pre-final year, having a lot of expertise in evaluating short answers. Each annotator was provided with comprehensive guidelines and requirements to execute their assigned task proficiently. Each evaluator was fairly compensated (5\$ per hour) for reviewing grades and the synthetically generated feedback. Each feedback from the randomly sampled 300     data points was scored independently, without access to the scores provided by each other. Human evaluation across various designed aspects, as mentioned in the quality estimate section, consistently yields an average score greater than \textbf{4.5 }out of \textbf{5}, which shows the high reliability of the feedback. 
The same annotators evaluate the correctness of each output label for sampled data points, achieving an accuracy of \textbf{98\%} and pair-wise average \textbf{Cohen's Kappa }($\kappa$) score of \textbf{0.65} (substantial agreement), showcasing the high reliability of the assigned output label.

\end{document}
